# Supplementary material for: Using BART to Perform Pareto Optimization and Quantify its Uncertainties
Source: arXiv:2101.02558 source file (2021-09-03)
Supplement: Supplementary file 1 [file SupplementaryMaterials.tex]

\bigskip
\begin{center}
{\large\bf APPENDIX A: PROOFS OF THEOREMS}
\end{center}

\begin{proof}[Proof of Theorem 1]
First we rewrite each single-output function $\ens(\bm{\cdot}; \theta_j)$ in (2) from the main text as a linear combination of indicator functions of hyperrectangles that partition the input space $\iset$. 
To do so, we pick an arbitrary $\ens(\bm{\cdot}; \theta_j)$ and, for notational ease, suppress the index $j$ so that $\ens(\bm{\cdot}; \theta_j) = \ens(\bm{\cdot}; \theta)$. 
Then $\ens(\bm{\cdot}; \theta)$ can be expressed as the sum in (4) of Horiguchi et al. (2021). 
For any tree $t$ in the ensemble, the hyperrectangle set $\{\R_{t, k} : k=1, \ldots, |\M_t|\}$ partitions the input space $\iset$. 
If we take any one hyperrectangle from each tree, the intersection of these $m$ hyperrectangles will also be a hyperrectangle, albeit possibly empty. 
Thus, the set of all such intersections, i.e. 
\begin{align*}
\Big\{\R_{1,k_1} \cap \R_{2,k_2} \cap \cdots \cap \R_{m,k_m} :
k_1 \in \{1, \ldots, |\M_1|\}, 
% k_2 \in \{1, \ldots, |\M_2|\}, 
\ldots,  
k_m \in \{1, \ldots, |\M_m|\}\Big\},
\end{align*} 
also partitions the input space. 
((5) of Pratola (2016) describes how to programatically implement this intersection.) % \mtp{Equation? or Appendix?}
For the single-output ensemble $\ens$, let $B_{\ens}$ index the set of the nonempty $m$-wise intersections. 
Then we may rewrite the function $\ens(\bm{\cdot}; \theta)$ as a linear combination of indicators\footnote{The indicator function $\1_{\R}(\bm{\cdot}): \iset \rightarrow \{0, 1\}$ of a hyperrectangle $\R \subset \iset$ is defined as follows: for an input $\x \in \iset$, the value $\1_{\R}(\x)$ equals one if $\x \in \R$ but equals zero if $\x \notin \R$.} of these nonempty intersections, i.e.
\begin{equation*}
\ens(\bm{\cdot}; \theta) = \sum_{l \in B_{\ens}} \alpha_l \1_{\R_l}(\bm{\cdot}),
\end{equation*}
where each $\alpha_l$ is the sum of the $m$ terminal node parameter values that correspond to the original hyperrectangles that created $\R_l$, i.e. if $\R_l = \R_{1,k_1} \cap \R_{2,k_2} \cap \cdots \cap \R_{m,k_m}$ then $\alpha_l = \mu_{1,k_1} + \mu_{2,k_2} + \cdots + \mu_{m,k_m}$.

Now we rewrite the $d-$objective ensemble function $\Ens(\bm{\cdot}; \bm{\theta})$, for which we bring back the previously suppressed index notation. 
For each ensemble $\ens_i$, the hyperrectangle set $\{\R_{l_i} : l_i \in B_{\ens_i}\}$ partitions the input space $\iset$. 
Similar to the previous paragraph, the set of all such $d-$wise intersections, i.e. 
\begin{align*}
\Big\{\R_{l_1} \cap \R_{l_2} \cap \cdots \cap \R_{l_d} :
l_1 \in B_{\ens_1}, 
l_2 \in B_{\ens_2}, 
\ldots,  
l_d \in B_{\ens_d}\Big\},
\end{align*} 
also partitions the input space, where each hyperrectangle $\R_{l_i}$ has associated with it the value $\alpha_{l_i}$. Hence, each $d-$wise intersection $\R_{l_1} \cap \R_{l_2} \cap \cdots \cap \R_{l_d}$ has associated with it the $d-$tuple $(\alpha_{l_1}, \alpha_{l_2}, \ldots, \alpha_{l_d}) \in \mathbb{R}^d$. 
For the multiple-output ensemble $\Ens$, let $B_{\Ens}$ index the set of the nonempty $d-$wise intersections. 
Then we may express the function $\Ens(\bm{\cdot}; \bm{\theta})$ as a linear combination of indicators of these nonempty intersections, i.e. 
\begin{equation*}
\Ens(\bm{\cdot}; \bm{\theta}) = \sum_{q \in B_{\Ens}} \bm{\alpha}_q \1_{\R_q}(\bm{\cdot}),
\end{equation*}
where each $\bm{\alpha}_q = (\alpha_{l_1}, \ldots, \alpha_{l_d}) \in \mathbb{R}^d$ when $\R_q = \R_{l_1} \cap \R_{l_2} \cap \cdots \cap \R_{l_d}$. 

\end{proof}

\newpage
\begin{center}
{\large\bf APPENDIX B: ALGORITHM PSEUDOCODE}
\end{center}

\subsection*{B.1 \quad Algorithm to find PF of a set of vectors.}

\begin{algorithm}[!ht]
\caption{Find the PF of a set of $d$-dimensional vectors.}
\label{alg:pfasensstep2}
\begin{algorithmic}[1]
\Require{Set $V = \{\vv_1, \ldots, \vv_{|V|}\}$ of $d$-dimensional vectors arranged in increasing order of their first coordinates. In case of ties, arrange elements in increasing order of their second coordinates. Repeat for further coordinates as necessary.} 
\Ensure{PF of $V$.}
\Statex
\State $PF \gets \textsc{FindPF}(V)$ 
\State 
\Function{FindPF}{$V$}
\State 
\If {$|V| == 1$}
\State
\Return $V$
\EndIf
\State 
\State Set $R \gets \textsc{FindPF}(\{\vv_1, \ldots, \vv_{\floor{|V|/2}}\})$ \texttt{ // recursive call}
\State Set $S \gets \textsc{FindPF}(\{\vv_{\floor{|V|/2}+1}, \ldots, \vv_{|V|}\})$ \texttt{ // recursive call}
\State
\State \texttt{// Create $T$ to be the set of vectors in $S$ not dominated by any vectors in $R$.}
\State Set $T \gets \emptyset$. 
\For{$\vv_i \in S$}
\If {$\vv_i \nprec R$}
\State Set $T \gets T \cup \{\vv_i\}$
\EndIf
\EndFor
\State
\State
\Return $R \cup T$
\State 
\EndFunction
\end{algorithmic}
\end{algorithm}

\subsection*{B.2 \quad Algorithm to compute modified band depth of CPFs for $d=2$.}

\noindent \textbf{Input:} CPFs $c^{(1)}, \ldots, c^{(N)}$, where $d=2$.

\noindent \textbf{Output:} Modified band depth of each CPF.

\begin{enumerate}
    \item Create cuts. (Time: $\mathcal{O}(N+q)$) 
    \begin{enumerate}
        \item Define endpoints for each axis. If the boundaries of the (rectangular) output space are known, for both $j \in \{1, 2\}$ denote $y_j^{min}$ ($y_j^{max}$) as the minimum (maximum) $j$th-dimensional boundary value. 
        Otherwise, for both $j \in \{1, 2\}$ let $y_j^{min}$ ($y_j^{max}$) be the minimum (maximum) $y_j$ value of the points in any of the $N$ CPFs. Then denote the intervals $I_1 := [y_1^{min}, y_1^{max}]$ and $I_2 := [y_2^{min}, y_2^{max}]$. 
        \item Create $q$ values $t_1, t_2, \ldots, t_q$ equally spaced in interval $I_1$, where $t_1=y_1^{min}$ and $t_q=y_1^{max}$. Similarly, create $q$ values $s_1, s_2, \ldots, s_q$ equally spaced in interval $I_2$, where $s_1=y_2^{min}$ and $s_q=y_2^{max}$.
    \end{enumerate}
    \item Create $(dq) \times N$ matrix $M$ by creating two $q \times N$ matrices $M^1$ and $M^2$, where the $ij$th element of $M^1$ is defined to be $h_1(t_i; c^{(j)}) := \min \{y_2 \in I_2 : (t_i, y_2) \in A^{(j)}\}$ and the $ij$th element of $M^2$ is defined to be $h_2(s_i; c^{(j)}) := \min \{y_1 \in I_1 : (y_1, s_i) \in A^{(j)}\}$. Matrix $M$ is the vertical stacking of matrices $M^1$ and $M^2$. (Time: $\mathcal{O}(q N)$) 
    \begin{enumerate}
        \item Put $\infty$ for the entries in the matrix $M$ corresponding to nonexistent values of $h_1(y_1; c^{(j)})$ or $h_2(y_2; c^{(j)})$.
    \end{enumerate}
    \item Create $(dq) \times N$ matrix $R^{\max}$ ($R^{\min}$) whose $i$th row is defined to be the ascending max (min) rank of the $i$th row of $M$, where ascending rank means the smallest value gets rank $1$ while the largest value gets rank $N$. (Time: $\mathcal{O}(q N \log N)$) 
    \item Create $(dq) \times N$ matrix $T$ whose $ij$th element is $T_{ij} = [R_{ij}^{\max}(N-R_{ij}^{\min}+1) - (R_{ij}^{\max}-R_{ij}^{\min}+1)^2]/\binom{N}{2}$, where $R_{ij}^{\max}$ ($R_{ij}^{\min}$) is the $ij$th element of the matrix $R^{\max}$ ($R^{\min}$). (Time: $\mathcal{O}(q N)$) 
    \item Create $N-$tuple whose $j$th element, defined to be the mean of the elements in matrix $T$'s $j$th column (i.e. $(2q)^{-1} \sum_{i=1}^{2q} T_{ij}$), is the depth of CPF $c^{(j)}$. (Time: $\mathcal{O}(q N)$) % as defined in Example (3) for CPF $c^{(*)}$.
\end{enumerate}

\subsection*{B.3 \quad Algorithm to compute modified band depth of CPFs for $d \geq 2$.}

\begin{figure}
    \centering
    \includegraphics[width=\textwidth]{../../Code/v_2/Plots/MBDd3Alg2.pdf} 
    \caption{Illustration of modified band depth algorithm for $d=3$. All objects in this objective space $\oset = [0,1]^3$ are projected onto a $2-$dimensional plane orthogonal to the 3rd principal axis. For simplicity, the three example CPFs each consist of a single point denoted by either a triangle (with coordinates $(0.4,0.1,2)$), square (with coordinates $(0.1,0.3,3)$), or star (with coordinates $(0.2,0.2,4)$). Their corresponding DPSCs are the areas with hatched lines. The uniform grid of circles represents the $q^{d-1} = 9^2$ lines parallel to the 3rd principal axis. (In practice, $q$ should be much larger than $9$.) The line $\{(0.5,0.5,x): x \in [0,1]\}$ intersects the triangle, square, and star DPSCs at third-coordinate values of, respectively, $2$, $3$, and $4$. Because $3$ lies strictly between $2$ and $4$, at this line the triangle, square, and star DPSCs have a band depth of, respectively, $2/3$, $1$, and $2/3$, which are computed in step 2 of the algorithm.}
    \label{fig:MBDd3Alg}
\end{figure}

The $d=2$ algorithm in B.2 is a special case of the algorithm described in this section, which accomodates any integer $d \geq 2$.
Assuming the output space is the Cartesian product of $d$ compact intervals, the idea is as follows: 
for every $k \in \{1, \ldots, d\}$, create a uniform grid of $q^{d-1}$ lines parallel to the $k$th principal axis of $\mathbb{R}^d$ and find the (univariate) CPF depths at each of these lines. 
Figure \ref{fig:MBDd3Alg} shows an illustration for when $k=d=3$ with two CPFs.
Each CPF will ultimately have $dq^{d-1}$ such depth values; the sample mean of these values will be the band depth of the CPF.

\noindent \textbf{Input:} CPFs $c^{(1)}, \ldots, c^{(N)}$, where $d \geq 2$.

\noindent \textbf{Output:} Modified band depth of each CPF.

\begin{enumerate}
    \item Create cuts. (Time: $\mathcal{O}(dN + dq^{d-1})$) 
    \begin{enumerate}
        \item Define the interval $I_k := [a_k, b_k]$ for each of the $k \in \{1, \ldots, d\}$ axes.
        \item Create the parallel lines. For each $k=1, \ldots, d$, create $q^{d-1}$ lines equally spaced in the $(d-1)-$dimensional surface $\prod_{i \neq k} I_i$.
        Define each line parallel to the $k$th principal axis as \[\{(y_1, \ldots, y_{k-1}, t, y_{k+1}, \ldots, y_d) : t \in \mathbb{R}\}\] for some set of $(d-1)$ values $\{y_i \in T_i\}_{i \neq k}$ where each $T_i$ is the set of $q$ values equally spaced in the interval $I_i$. 
    \end{enumerate}
    \item Create $(dq^{d-1}) \times N$ matrix $M$ by creating $q^{d-1} \times N$ matrices $M^1, \ldots, M^d$, where the $ij$th element of each matrix $M^k$ is defined to be the $y_k$ value where CPF $c^{(j)}$ intersects line $i \in \{1, \ldots, q^{d-1}\}$ parallel to the $k$th principal axis. Matrix $M$ is the vertical stacking of the matrices $M^1, \ldots, M^d$. (Time: $\mathcal{O}(d q^{d-1} N)$) 
    \begin{enumerate}
        \item Put $\infty$ for the entries where $c^{(j)}$ doesn't intersect line $i$.
    \end{enumerate}
    \item Create $(dq^{d-1}) \times N$ matrix $R^{\max}$ ($R^{\min}$) whose $i$th row is defined to be the ascending max (min) rank of the $i$th row of $M$, where ascending rank means the smallest value gets rank $1$ while the largest value gets rank $N$. (Time: $\mathcal{O}(d q^{d-1} N \log N)$) 
    \item Create $(dq^{d-1}) \times N$ matrix $T$ whose $ij$th element is $T_{ij} = [R_{ij}^{\max}(N-R_{ij}^{\min}+1) - (R_{ij}^{\max}-R_{ij}^{\min}+1)^2]/\binom{N}{2}$, where $R_{ij}^{\max}$ ($R_{ij}^{\min}$) is the $ij$th element of the matrix $R^{\max}$ ($R^{\min}$). (Time: $\mathcal{O}(d q^{d-1} N)$) 
    \item Create $N-$tuple whose $j$th element, defined to be the mean of the elements in matrix $T$'s $j$th column (i.e. $(dq^{d-1})^{-1} \sum_{i=1}^{dq^{d-1}} T_{ij}$), is the depth of CPF $c^{(j)}$. (Time: $\mathcal{O}(d q^{d-1} N)$) 
\end{enumerate}

\newpage
\begin{center}
{\large\bf APPENDIX C: TEST FUNCTION DEFINITIONS}
\end{center}

% \subsection*{Test function definitions}

\begin{enumerate}
    \item MOP2 from Fonseca and Fleming (1995) has $p=2$ inputs and $d=2$ objectives:
    \begin{align*}
      f_1(\mathbf{x}) &= 1 - \exp\left\{-\sum_{i=1}^2 \left(4x_i - 2 - \frac{1}{\sqrt{2}}\right)^2\right\} \\
      f_2(\mathbf{x}) &= 1 - \exp\left\{-\sum_{i=1}^2 \left(4x_i - 2 + \frac{1}{\sqrt{2}}\right)^2\right\}.
    \end{align*} 
    The PS is the line segment $\pstrue = \{(t, t) : (2-1/\sqrt{2})/4 \leq t \leq (2+1/\sqrt{2})/4\}$ and the PF is the concave curve segment shown in Figure 5 of the main text.
    Also, $\Var_{\X}(f_1(\X)) = \Var_{\X}(f_2(\X)) \approx 0.0636$.
    \item ZDT3 from Zitzler et al. (2000) has a disconnected PF and PS. For $p = 2$ inputs, the $d=2$ objectives are
    \begin{align*}
      f_1(\mathbf{x}) &= x_1 \\
      f_2(\mathbf{x}) &= \left[\left(1 - \sqrt{x_1 / g}\right) - \frac{x_1}{g} \sin(10 \pi x_1) + c_3\right] / (10 + c_3),
    \end{align*}
    where $c_3 := 0.70238$ and $g := 1 + \frac{9}{p-1} \sum_{i=2}^p x_i = 1 + 9 x_2$. 
    Figure 5 of the main text shows the PF and PS.
    Also, $\Var_{\X}(f_1(\X)) = \frac{1}{12} \approx 0.0833$ and $\Var_{\X}(f_2(\X)) \approx 0.0461$. 
    \item We modify DTLZ2 from Deb et al. (2005) for $p=4$ inputs and $d=2$ objectives so that the resulting PF is convex rather than concave. 
    Our modified objectives are 
    \begin{align*}
      f_1(\mathbf{x}) &= \left(g(\x_{2:4}) - 1\right) \cos\left(\frac{\pi x_1}{2}\right) + 1 \\
      f_2(\mathbf{x}) &= \left(g(\x_{2:4}) - 1\right) \sin\left(\frac{\pi x_1}{2}\right) + 1, 
    \end{align*}
    where $g(\x_{2:4}) := \sum_{i=2}^4 (x_i - 0.5)^2$.
    The PS is the line segment $\pstrue = \{(x_1, 0.5, 0.5, 0.5): x_1 \in [0, 1]\}$ and the PF is the convex quarter-circle $\pftrue = \{(1-\cos t, 1-\sin t) : t \in [0, \pi/2]\}$ shown in Figure 5 of the main text. 
    Also, $\Var_{\X}(f_1(\X)) = \Var_{\X}(f_2(\X)) \approx 0.0616$. 
    \item We modify ZLT1 from Laumanns (2005) to have $p=10$ inputs, with seven of them inert, and $d=3$ objectives: 
    \begin{equation*}
      f_i(\mathbf{x}) = 0.2 \times \left\{ 0.5(x_i-1)^2 + \sum_{\substack{j=1 \\ j\neq i}}^3 x_i^2 \right\} \quad \quad i=1,2,3
    \end{equation*}
    The PS is the $(p-1)-$dimensional hyperplane $\pstrue = \{\x: \sum_{j=1}^3 x_i = 1 \}$ and the PF (shown in Figure 5 of the main text) is convex.
    Also, $\Var_{\X}(f_1(\X)) = \Var_{\X}(f_2(\X)) = \Var_{\X}(f_3(\X)) =0.032$. 
\end{enumerate}

\newpage
\begin{center}
{\large\bf APPENDIX D: SIMULATION STUDY FULL RESULTS}
\end{center}

See Figures \ref{fig:resultsMOP2}, \ref{fig:resultsZDT3}, and \ref{fig:resultsDTLZ2}.

\begin{figure}
    \centering
    \begin{subfigure}[t]{\textwidth}
        \centering
        \includegraphics[width=\textwidth]{../../Code/v_2/Plots/Results/MOP2pf.pdf} 
        \caption{MOP2 PF data.}
        \label{fig:resMOP2pf}
    \end{subfigure}
    ~
    \begin{subfigure}[t]{\textwidth}
        \centering
        \includegraphics[width=\textwidth]{../../Code/v_2/Plots/Results/MOP2ps.pdf} 
        \caption{MOP2 PS data.}
        \label{fig:resMOP2ps}
    \end{subfigure}
    \caption{Bagplots of the 100 values of $d(\phat, \ptrue)$ and $d(\ptrue, \phat)$ for both the PF and PS. Each plot represents a simulation scenario where $n \in \{64, 128\}$, and the variance multiplier is a value in $\{0, 0.1, 0.25\}$. Bags with solid (dashed) outline and median labeled `d' (`r') display depth (random sets) approach. Black (gray) bags display BART (GP) model.}
    \label{fig:resultsMOP2}
\end{figure}

\begin{figure}
    \centering
    \begin{subfigure}[t]{\textwidth}
        \centering
        \includegraphics[width=\textwidth]{../../Code/v_2/Plots/Results/ZDT3pf.pdf} 
        \caption{ZDT3 PF data.}
        \label{fig:resZDT3pf}
    \end{subfigure}
    ~
    \begin{subfigure}[t]{\textwidth}
        \centering
        \includegraphics[width=\textwidth]{../../Code/v_2/Plots/Results/ZDT3ps.pdf} 
        \caption{ZDT3 PS data.}
        \label{fig:resZDT3ps}
    \end{subfigure}
    \caption{Bagplots of the 100 values of $d(\phat, \ptrue)$ and $d(\ptrue, \phat)$ for both the PF and PS. Each plot represents a simulation scenario where $n \in \{64, 128\}$, and the variance multiplier is a value in $\{0, 0.1, 0.25\}$. Bags with solid (dashed) outline and median labeled `d' (`r') display depth (random sets) approach. Black (gray) bags display BART (GP) model.}
    \label{fig:resultsZDT3}
\end{figure}

\begin{figure}
    \centering
    \begin{subfigure}[t]{\textwidth}
        \centering
        \includegraphics[width=\textwidth]{../../Code/v_2/Plots/Results/DTLZ2pf.pdf} 
        \caption{DTLZ2 PF data.}
        \label{fig:resDTLZ2pf}
    \end{subfigure}
    ~
    \begin{subfigure}[t]{\textwidth}
        \centering
        \includegraphics[width=\textwidth]{../../Code/v_2/Plots/Results/DTLZ2ps.pdf} 
        \caption{DTLZ2 PS data.}
        \label{fig:resDTLZ2ps}
    \end{subfigure}
    \caption{Bagplots of the 100 values of $d(\phat, \ptrue)$ and $d(\ptrue, \phat)$ for both the PF and PS. Each plot represents a simulation scenario where $n \in \{128, 256\}$, and the variance multiplier is a value in $\{0, 0.1, 0.25\}$. Bags with solid (dashed) outline and median labeled `d' (`r') display depth (random sets) approach. Black (gray) bags display BART (GP) model.}
    \label{fig:resultsDTLZ2}
\end{figure}

\begin{figure}
    \centering
    \begin{subfigure}[t]{\textwidth}
        \centering
        \includegraphics[width=\textwidth]{../../Code/v_2/Plots/Results/ZLT1pf.pdf} 
        \caption{ZLT1 PF data.}
        \label{fig:resZLT1pf}
    \end{subfigure}
    ~
    \begin{subfigure}[t]{\textwidth}
        \centering
        \includegraphics[width=\textwidth]{../../Code/v_2/Plots/Results/ZLT1ps.pdf} 
        \caption{ZLT1 PS data.}
        \label{fig:resZLT1ps}
    \end{subfigure}
    \caption{Bagplots of the 50 values of $d(\phat, \ptrue)$ and $d(\ptrue, \phat)$ for both the PF and PS. Each plot represents a simulation scenario where $n \in \{96, 192\}$, and the variance multiplier is a value in $\{0, 0.1, 0.25\}$. Bags with solid (dashed) outline and median labeled `d' (`r') display depth (random sets) approach. Black bags display BART model.}
    \label{fig:resultsZLT1}
\end{figure}
